# Supplementary material for: Temporal Betweenness Centrality on Shortest Walks Variants
Source: arXiv:2305.01080 source file (2024-02-12)
Supplement: Supplementary file 1 [file appendix_not_paper.tex]

\begin{algorithm}[H]
     \begin{algorithmic}[1]

    \Require  $G = (V,\E,T)$ : a temporal graph, $G_s$ the predecessor graph of $s$ 
    \Ensure $\delta_{s\bullet}(v,t), \forall v \in V, t \in T$
    \Function{General\_Contribution}{$G_s, s$}
    \State $\sigma_{sz}^{\W},\delta_{sv}(v,t), \sigma_{s,(v,t)}= \textsc{count\_walks}(G,s)$ 
    \State $\delta_{s\bullet}(v,t) = 0, \forall v \in V, t \in T$
    \State $visited = \{\}$
    \For{$(v,t) \in sources(G_s)$}
    \State $\textsc{general\_rec}((v,t),\delta_{s\bullet},\sigma_{sz},\delta_{sv}(v,t), \sigma_{s,(v,t)} )$
    \EndFor
 \textbf{return} $\delta_{s\bullet}(v,t), \delta_{sv}(v,t)$
    \EndFunction
  \end{algorithmic}
 	\begin{algorithmic}[1]
    \Function{General\_rec}{$(v,t),\delta_{s\bullet},\sigma_{sz},\delta_{sv}(v,t), \sigma_{s,(v,t)}$}
    \If{$(v,t)$ not in visited}
    \State $su = 0$
    \For{$  t' \in \{t'' | \exists ((v,t), (w,t'')) \in E_s \}  $, in decreasing order}
    \For{$ w \in \{((v,t),(w,t')) \in E_s  \}$}
    \State \textsc{General\_rec}{$((w,t'),\delta_{s\bullet},\sigma_{sz},\delta_{sv}(v,t), \sigma_{s,(v,t)})$}
    \State $su = su + \dfrac{\sigma_{s,(v,t)}}{\sigma_{s,(w,t')}} \delta_{s\bullet}(w,t')$
    \EndFor
    \State $\textsc{interm\_contribution}((v,t),t',su)$ \Comment{for passive walks ignore this}
    \EndFor
    \State $\delta_{s\bullet}(v,t) = su + \delta_{sv}(v,t)$
    \State $visited.\textsc{add}((v,t))$
    \EndIf
    \EndFunction
  \end{algorithmic}
  	\caption{\label{algo:general_contribution} Compute the values of $\delta_{s\bullet}(v,t)$ for a temporal graph $G$}
\end{algorithm}
 
\begin{algorithm}[H]
	\caption{\label{algo:betweenness} Computes the values of $B(v,t)$ for all temporal nodes in a graph $G$}
	\begin{algorithmic}[1]

    \Require  $G = (V,\E,T)$ : a temporal graph 
    \Ensure $B(v,t), \forall v \in V, t \in T$
    \Function{Betweenness}{$G$}
    \For {$s \in V$}
    \State $B(v,t) = 0, \forall v\in V, t \in T$
    \State $G_s$ = \textsc{Temporal\_BFS}$(G, s)$
    \State $\delta_{s\bullet}(v,t), \delta_{sv}^{\W}(v,t)$ = \textsc{General\_Contribution}$(G_s,s)$
    \State \textsc{Update\_betweenness}$(B(v,t), \delta_{s\bullet}(v,t),\delta_{sv}(v,t))$ \Comment{Applies Equation~\eqref{eq:hat_b}}
    \EndFor
 \textbf{return} $B(v,t)$
    \EndFunction
  \end{algorithmic}
\end{algorithm}

\begin{algorithm}[h!]
	\caption{\label{algo:general_rec} Intermediary contribution}
	\begin{algorithmic}[1]
    \Function{inter\_contribution}{$G_s, (v,t),t', sum$} 
    %\State $t'' = next\_event(t)$; \Comment{returns next time or $-1$ if it is the last event time}
    \State $t'' = t'$
        \While{$t'' \geq t$ and $before_{G_s}(v,t'') = t$ and $(v,t'') \notin visited$}
        \State $\delta_{s\bullet}(v,t'') = \delta_{sv}(v,t'') + sum$
        \State $visited.\textsc{add}((v,t''))$
%    \For{$t \in \{ t'' | t'' \in event\_times, t < t'' \leq t', (v,t'') \notin V_s \} $ in increasing order}
    \State $t'' = previous\_event(t'')$ 
    \EndWhile
    \EndFunction
  \end{algorithmic}
\end{algorithm}
